# Supplementary material for: Simultaneous emission from dust and gas in the planetary debris orbiting a white dwarf
Source: arXiv:2412.07647 source file (2024-12-10)
Supplement: Supplementary file 1 [file Supplementary_Tables.pdf]

**Table A1.** The dates at which X-shooter and HAWKI data were taken; if the two sets of data were taken within 4 days of each other, they are reported on the same row. The SNR for the X-shooter data is reported for both the UVB and VIS arms with each exposure reported separately if more than one is available. The HAWKI $J$, $H$ and $Ks$ magnitudes are reported with errors for differential photometry. If absolutely calibrated magnitudes are required, add the following errors in quadrature with the reported errors: $J$: 0.01 mags, $H$: 0.02 mags, $Ks$: 0.02 mags.

| Date X-shooter | SNR UVB | SNR VIS | Date HAWKI | J (mag) | H (mag) | $Ks$ (mag) |
|---|---|---|---|---|---|---|
| 2019 Oct 10 | 152.7/159.9 | 84.6/89.1 | | | | |
| 2021 June 28 | 149.2/161.9 | 82.2/87.7 | | | | |
| | | | 2022 Apr 29 | 15.679 ± 0.006 | 15.604 ± 0.009 | 15.110 ± 0.009 |
| 2022 Apr 30 | 95.6/101.1 | 53.7/56.5 | 2022 Apr 30 | 15.684 ± 0.006 | 15.614 ± 0.009 | 15.157 ± 0.009 |
| 2022 May 24 | 115.9/111.2 | 64.1/61.5 | | | | |
| 2022 May 26 | 325.6 | 174.5 | 2022 May 26 | 15.717 ± 0.006 | 15.698 ± 0.010 | 15.308 ± 0.009 |
| 2022 May 31 | 111.4/109.5 | 61.8/60.5 | 2022 May 31 | 15.700 ± 0.006 | 15.670 ± 0.009 | 15.212 ± 0.009 |
| | | | 2022 June 12 | 15.717 ± 0.006 | 15.696 ± 0.010 | 15.308 ± 0.009 |
| 2022 July 03 | 115.0/116.4 | 64.0/65.2 | 2022 July 04 | 15.715 ± 0.006 | 15.700 ± 0.010 | 15.305 ± 0.009 |
| 2022 July 26 | 88.2/93.9 | 49.3/52.3 | 2022 July 26 | 15.709 ± 0.006 | 15.696 ± 0.010 | 15.290 ± 0.009 |
| 2022 Aug 13 | 89.9/95.8 | 47.5/50.3 | | | | |
| 2022 Aug 14 | 111.3/106.5 | 61.4/58.9 | 2022 Aug 15 | 15.713 ± 0.006 | 15.716 ± 0.010 | 15.291 ± 0.009 |
| 2022 Sep 20 | 119.7/114.1 | 64.7/62.5 | 2022 Sept 20 | 15.713 ± 0.006 | 15.710 ± 0.010 | 15.276 ± 0.009 |
| 2022 Sep 30 | 127.0/125.9 | 69.5/69.1 | 2022 Sept 30 | 15.708 ± 0.006 | 15.708 ± 0.010 | 15.272 ± 0.009 |
| 2022 Oct 02 | 114.9/113.3 | 62.8/62.0 | 2022 Oct 02 | 15.716 ± 0.006 | 15.699 ± 0.010 | 15.288 ± 0.009 |
| 2022 Oct 25 | 116.8/113.9 | 64.0/62.6 | 2022 Oct 24 | 15.714 ± 0.006 | 15.687 ± 0.010 | 15.303 ± 0.009 |
| 2023 Apr 11 | 86.0/92.4 | 52.0/55.8 | | | | |
| 2023 May 02 | 377.7 | 211.1 | | | | |
| 2023 May 12 | 110.9/113.0 | 59.9/61.3 | 2023 May 16 | 15.711 ± 0.006 | 15.681 ± 0.010 | 15.267 ± 0.009 |
| | | | 2023 May 18 | 15.713 ± 0.006 | 15.710 ± 0.010 | 15.276 ± 0.009 |
| 2023 May 23 | 126.9/126.8 | 68.7/68.5 | 2023 May 22 | 15.714 ± 0.006 | 15.696 ± 0.010 | 15.271 ± 0.009 |
| | | | 2023 May 25 | 15.710 ± 0.006 | 15.683 ± 0.010 | 15.258 ± 0.009 |
| 2023 June 08 | 91.5/89.2 | 69.6/68.2 | | | | |
| 2023 June 15 | 122.6/125.0 | 66.7/68.2 | 2023 June 13 | 15.713 ± 0.006 | 15.670 ± 0.010 | 15.240 ± 0.009 |
| 2023 June 22 | 122.6/120.7 | 66.3/65.0 | 2023 June 22 | 15.707 ± 0.006 | 15.657 ± 0.009 | 15.174 ± 0.009 |
| | | | 2023 July 07 | 15.712 ± 0.006 | 15.680 ± 0.010 | 15.254 ± 0.009 |
| 2023 July 18 | 114.4/120.2 | 60.1/62.9 | | | | |
| 2023 Aug 05 | 112.7/116.8 | 62.9/65.0 | 2023 Aug 05 | 15.690 ± 0.006 | 15.617 ± 0.009 | 15.136 ± 0.009 |
| 2023 Aug 18 | 116.9/111.0 | 64.0/60.8 | 2023 Aug 21 | 15.717 ± 0.006 | 15.703 ± 0.010 | 15.263 ± 0.009 |
| 2023 Sep 06 | 107.3/102.6 | 57.4/55.7 | 2023 Sept 06 | 15.709 ± 0.006 | 15.711 ± 0.011 | 15.261 ± 0.010 |
| 2023 Sep 17 | 122.3/123.3 | 66.4/67.1 | 2023 Sept 13 | 15.718 ± 0.006 | 15.726 ± 0.010 | 15.310 ± 0.010 |
| 2023 Sep 20 | 118.0/121.9 | 65.0/67.3 | 2023 Sept 20 | 15.719 ± 0.006 | 15.714 ± 0.010 | 15.307 ± 0.009 |

**Table A2.** The X-shooter line fluxes (in $10^{-13}\,\mathrm{ergs\,cm^{-2}\,s^{-1}}$) for the gaseous emission lines.

| MJD | Fe 5275 | Fe 5316 | O 7774 | O 8446 | Ca 8500 | Ca 8545 | Ca 8660 | Mg 8806 |
|---|---|---|---|---|---|---|---|---|
| 58766.06648 | $27.8 \pm 1.1$ | $56.50 \pm 0.97$ | $9.47 \pm 0.68$ | $9.7 \pm 1.0$ | $8.64 \pm 0.54$ | $4.98 \pm 0.48$ | $4.72 \pm 0.49$ | $3.53 \pm 0.34$ |
| 58766.08718 | $39.2 \pm 1.1$ | $48.83 \pm 0.92$ | $9.72 \pm 0.65$ | $5.92 \pm 0.99$ | $8.54 \pm 0.51$ | $5.51 \pm 0.46$ | $3.28 \pm 0.46$ | $3.38 \pm 0.33$ |
| 59393.25132 | $29.0 \pm 1.1$ | $50.66 \pm 0.98$ | $4.49 \pm 0.68$ | $12.1 \pm 1.0$ | $8.85 \pm 0.55$ | $4.28 \pm 0.48$ | $6.33 \pm 0.52$ | $1.71 \pm 0.36$ |
| 59393.27201 | $23.2 \pm 1.1$ | $47.14 \pm 0.90$ | $4.09 \pm 0.64$ | $17.85 \pm 0.98$ | $10.87 \pm 0.53$ | $5.35 \pm 0.45$ | $4.71 \pm 0.49$ | $4.22 \pm 0.35$ |
| 59699.35677 | $42.2 \pm 1.7$ | $52.4 \pm 1.5$ | $15.9 \pm 1.1$ | $10.9 \pm 1.4$ | $35.51 \pm 0.85$ | $45.99 \pm 0.78$ | $36.76 \pm 0.92$ | $8.01 \pm 0.56$ |
| 59699.36405 | $47.2 \pm 1.7$ | $60.3 \pm 1.4$ | $10.1 \pm 1.0$ | $9.8 \pm 1.4$ | $37.89 \pm 0.81$ | $45.10 \pm 0.74$ | $38.26 \pm 0.85$ | $6.28 \pm 0.53$ |
| 59723.31152 | $49.2 \pm 1.5$ | $54.9 \pm 1.3$ | $10.56 \pm 0.88$ | $15.1 \pm 1.1$ | $23.97 \pm 0.70$ | $21.32 \pm 0.64$ | $18.83 \pm 0.66$ | $5.30 \pm 0.47$ |
| 59723.31879 | $37.5 \pm 1.5$ | $55.1 \pm 1.3$ | $4.89 \pm 0.92$ | $16.5 \pm 1.3$ | $27.21 \pm 0.72$ | $25.11 \pm 0.67$ | $18.67 \pm 0.69$ | $5.15 \pm 0.48$ |
| 59725.38037 | $34.44 \pm 0.52$ | $58.69 \pm 0.44$ | $11.55 \pm 0.34$ | $13.62 \pm 0.60$ | $18.17 \pm 0.31$ | $16.37 \pm 0.26$ | $13.93 \pm 0.36$ | $2.77 \pm 0.18$ |
| 59730.29845 | $38.8 \pm 1.5$ | $55.0 \pm 1.3$ | $9.25 \pm 0.92$ | $11.8 \pm 1.2$ | $10.60 \pm 0.71$ | $8.45 \pm 0.66$ | $9.91 \pm 0.77$ | $3.31 \pm 0.48$ |
| 59730.30573 | $24.4 \pm 1.5$ | $57.3 \pm 1.3$ | $12.60 \pm 0.94$ | $16.4 \pm 1.2$ | $13.13 \pm 0.73$ | $8.91 \pm 0.67$ | $9.34 \pm 0.82$ | $4.76 \pm 0.49$ |
| 59763.32181 | $36.6 \pm 1.5$ | $51.7 \pm 1.3$ | $13.15 \pm 0.88$ | $17.6 \pm 1.0$ | $11.34 \pm 0.66$ | $5.21 \pm 0.62$ | $5.57 \pm 0.65$ | $0.69 \pm 0.47$ |
| 59763.32908 | $39.6 \pm 1.5$ | $53.3 \pm 1.3$ | $12.58 \pm 0.87$ | $14.75 \pm 0.98$ | $11.29 \pm 0.65$ | $6.19 \pm 0.61$ | $5.00 \pm 0.64$ | $4.09 \pm 0.46$ |
| 59786.11357 | $33.9 \pm 1.9$ | $60.3 \pm 1.6$ | $10.3 \pm 1.1$ | $11.0 \pm 1.7$ | $7.68 \pm 0.88$ | $6.32 \pm 0.81$ | $2.44 \pm 0.85$ | $3.83 \pm 0.61$ |
| 59786.12085 | $26.0 \pm 1.8$ | $52.3 \pm 1.5$ | $8.0 \pm 1.1$ | $8.0 \pm 1.4$ | $7.12 \pm 0.86$ | $5.66 \pm 0.76$ | $3.98 \pm 0.80$ | $3.54 \pm 0.57$ |
| 59804.20160 | $21.1 \pm 1.9$ | $48.2 \pm 1.6$ | $7.8 \pm 1.2$ | $16.5 \pm 1.5$ | $7.48 \pm 0.93$ | $2.41 \pm 0.85$ | $4.59 \pm 0.88$ | $2.57 \pm 0.64$ |
| 59804.20890 | $23.2 \pm 1.8$ | $48.1 \pm 1.5$ | $11.5 \pm 1.1$ | $13.9 \pm 1.4$ | $8.51 \pm 0.87$ | $5.46 \pm 0.80$ | $4.84 \pm 0.82$ | $0.88 \pm 0.61$ |
| 59805.16578 | $25.3 \pm 1.5$ | $51.3 \pm 1.3$ | $11.56 \pm 0.92$ | $9.4 \pm 1.1$ | $6.44 \pm 0.71$ | $3.94 \pm 0.67$ | $6.01 \pm 0.64$ | $1.29 \pm 0.48$ |
| 59805.17305 | $24.8 \pm 1.6$ | $52.1 \pm 1.4$ | $3.41 \pm 0.96$ | $10.1 \pm 1.1$ | $6.95 \pm 0.73$ | $1.75 \pm 0.69$ | $3.48 \pm 0.67$ | $4.66 \pm 0.50$ |
| 59842.11708 | $25.8 \pm 1.4$ | $48.0 \pm 1.2$ | $11.66 \pm 0.90$ | $12.9 \pm 1.3$ | $7.56 \pm 0.68$ | $3.35 \pm 0.62$ | $2.89 \pm 0.63$ | $1.56 \pm 0.46$ |
| 59842.12435 | $14.2 \pm 1.5$ | $54.8 \pm 1.3$ | $16.19 \pm 0.94$ | $9.2 \pm 1.2$ | $4.82 \pm 0.70$ | $1.64 \pm 0.64$ | $7.46 \pm 0.66$ | $3.44 \pm 0.48$ |
| 59852.03120 | $20.4 \pm 1.3$ | $47.9 \pm 1.2$ | $4.19 \pm 0.84$ | $14.0 \pm 1.2$ | $6.50 \pm 0.63$ | $1.54 \pm 0.58$ | $4.77 \pm 0.58$ | $-0.04 \pm 0.43$ |
| 59852.03848 | $18.5 \pm 1.4$ | $55.3 \pm 1.2$ | $9.69 \pm 0.85$ | $6.87 \pm 0.99$ | $6.44 \pm 0.64$ | $1.57 \pm 0.58$ | $5.34 \pm 0.62$ | $0.68 \pm 0.43$ |
| 59854.09335 | $37.7 \pm 1.5$ | $52.5 \pm 1.3$ | $9.32 \pm 0.95$ | $8.9 \pm 1.1$ | $6.36 \pm 0.69$ | $2.95 \pm 0.65$ | $3.63 \pm 0.68$ | $3.70 \pm 0.47$ |
| 59854.10064 | $33.7 \pm 1.5$ | $50.5 \pm 1.3$ | $11.91 \pm 0.96$ | $17.2 \pm 1.2$ | $8.74 \pm 0.70$ | $4.88 \pm 0.66$ | $3.35 \pm 0.69$ | $1.06 \pm 0.48$ |
| 59877.04943 | $20.8 \pm 1.4$ | $50.7 \pm 1.2$ | $7.64 \pm 0.93$ | $15.9 \pm 1.3$ | $11.90 \pm 0.71$ | $5.70 \pm 0.64$ | $7.09 \pm 0.67$ | $1.52 \pm 0.46$ |
| 59877.05670 | $28.3 \pm 1.5$ | $48.8 \pm 1.3$ | $7.01 \pm 0.95$ | $14.4 \pm 1.4$ | $12.0 \pm 0.85$ | $4.15 \pm 0.65$ | $4.26 \pm 0.70$ | $1.75 \pm 0.47$ |
| 60045.38762 | $26.8 \pm 1.9$ | $50.6 \pm 1.6$ | $8.3 \pm 1.1$ | $11.0 \pm 1.4$ | $9.95 \pm 0.83$ | $5.58 \pm 0.76$ | $6.82 \pm 0.93$ | $2.14 \pm 0.55$ |
| 60045.39524 | $33.3 \pm 1.8$ | $69.4 \pm 1.5$ | $10.0 \pm 1.0$ | $15.9 \pm 1.3$ | $8.78 \pm 0.77$ | $3.42 \pm 0.73$ | $5.51 \pm 0.83$ | $1.68 \pm 0.52$ |
| 60066.36953 | $30.13 \pm 0.44$ | $51.58 \pm 0.38$ | $9.28 \pm 0.27$ | $8.48 \pm 0.44$ | $7.40 \pm 0.21$ | $3.76 \pm 0.20$ | $2.47 \pm 0.21$ | $2.63 \pm 0.14$ |
| 60076.39601 | $30.8 \pm 1.5$ | $57.3 \pm 1.3$ | $8.45 \pm 0.95$ | $10.2 \pm 1.4$ | $4.76 \pm 0.75$ | $3.20 \pm 0.69$ | $6.31 \pm 0.75$ | $-0.96 \pm 0.49$ |
| 60076.40363 | $33.5 \pm 1.5$ | $42.7 \pm 1.3$ | $9.87 \pm 0.93$ | $12.3 \pm 1.1$ | $10.72 \pm 0.74$ | $6.55 \pm 0.67$ | $4.50 \pm 0.74$ | $2.89 \pm 0.48$ |
| 60087.38892 | $38.6 \pm 1.3$ | $46.5 \pm 1.1$ | $7.51 \pm 0.81$ | $10.48 \pm 0.96$ | $6.37 \pm 0.63$ | $2.63 \pm 0.60$ | $5.96 \pm 0.69$ | $2.10 \pm 0.43$ |
| 60087.39656 | $30.8 \pm 1.3$ | $49.8 \pm 1.2$ | $9.57 \pm 0.82$ | $11.3 \pm 1.0$ | $7.27 \pm 0.65$ | $3.59 \pm 0.59$ | $4.23 \pm 0.64$ | $2.19 \pm 0.43$ |
| 60103.40200 | $26.1 \pm 1.8$ | $48.2 \pm 1.6$ | $7.39 \pm 0.82$ | $13.9 \pm 1.1$ | $10.94 \pm 0.65$ | $5.65 \pm 0.59$ | $3.62 \pm 0.65$ | $1.98 \pm 0.42$ |
| 60103.41000 | $18.2 \pm 1.9$ | $48.8 \pm 1.6$ | $7.35 \pm 0.84$ | $8.4 \pm 1.2$ | $7.58 \pm 0.67$ | $2.81 \pm 0.61$ | $3.84 \pm 0.63$ | $0.32 \pm 0.43$ |
| 60110.33391 | $29.3 \pm 1.4$ | $52.1 \pm 1.2$ | $5.43 \pm 0.84$ | $12.7 \pm 1.1$ | $7.46 \pm 0.66$ | $4.00 \pm 0.61$ | $3.45 \pm 0.65$ | $1.90 \pm 0.44$ |
| 60110.34153 | $23.0 \pm 1.4$ | $47.8 \pm 1.2$ | $1.91 \pm 0.82$ | $10.3 \pm 1.1$ | $6.85 \pm 0.64$ | $4.15 \pm 0.60$ | $4.53 \pm 0.69$ | $5.59 \pm 0.43$ |
| 60117.30773 | $11.6 \pm 1.4$ | $54.0 \pm 1.2$ | $12.58 \pm 0.85$ | $8.9 \pm 1.1$ | $7.70 \pm 0.67$ | $3.96 \pm 0.62$ | $4.90 \pm 0.65$ | $0.24 \pm 0.45$ |
| 60117.31535 | $22.0 \pm 1.4$ | $48.4 \pm 1.2$ | $6.90 \pm 0.87$ | $13.5 \pm 1.0$ | $9.40 \pm 0.69$ | $5.75 \pm 0.62$ | $3.82 \pm 0.65$ | $2.17 \pm 0.45$ |
| 60143.19602 | $31.9 \pm 1.5$ | $51.3 \pm 1.3$ | $11.12 \pm 0.95$ | $12.7 \pm 1.3$ | $8.88 \pm 0.74$ | $4.60 \pm 0.68$ | $4.00 \pm 0.67$ | $-1.12 \pm 0.49$ |
| 60143.20364 | $22.9 \pm 1.4$ | $55.7 \pm 1.2$ | $10.93 \pm 0.91$ | $13.1 \pm 1.1$ | $9.92 \pm 0.72$ | $5.30 \pm 0.66$ | $4.00 \pm 0.63$ | $0.36 \pm 0.47$ |
| 60161.21424 | $53.2 \pm 1.5$ | $62.5 \pm 1.3$ | $15.20 \pm 0.90$ | $16.1 \pm 1.2$ | $36.06 \pm 0.72$ | $43.34 \pm 0.65$ | $35.75 \pm 0.64$ | $9.63 \pm 0.47$ |
| 60161.22187 | $44.7 \pm 1.4$ | $63.1 \pm 1.2$ | $10.25 \pm 0.87$ | $16.0 \pm 1.0$ | $33.65 \pm 0.67$ | $41.62 \pm 0.63$ | $38.48 \pm 0.62$ | $4.82 \pm 0.45$ |
| 60174.23020 | $44.9 \pm 1.4$ | $53.9 \pm 1.2$ | $17.31 \pm 0.89$ | $18.3 \pm 1.2$ | $13.14 \pm 0.67$ | $7.68 \pm 0.62$ | $6.45 \pm 0.68$ | $3.55 \pm 0.46$ |
| 60174.23782 | $30.1 \pm 1.5$ | $58.4 \pm 1.3$ | $7.73 \pm 0.94$ | $13.0 \pm 1.1$ | $11.26 \pm 0.71$ | $5.41 \pm 0.66$ | $4.47 \pm 0.71$ | $1.02 \pm 0.48$ |
| 60193.09715 | $32.4 \pm 1.6$ | $61.6 \pm 1.3$ | $15.0 \pm 1.0$ | $12.4 \pm 1.4$ | $9.00 \pm 0.77$ | $7.15 \pm 0.71$ | $4.68 \pm 0.75$ | $1.21 \pm 0.51$ |
| 60193.10477 | $28.2 \pm 1.6$ | $60.7 \pm 1.4$ | $8.6 \pm 1.1$ | $16.5 \pm 1.4$ | $11.59 \pm 0.82$ | $6.10 \pm 0.73$ | $3.92 \pm 0.74$ | $-0.76 \pm 0.53$ |
| 60204.07595 | $28.6 \pm 1.4$ | $54.8 \pm 1.2$ | $10.40 \pm 0.90$ | $13.8 \pm 1.1$ | $9.38 \pm 0.73$ | $4.92 \pm 0.62$ | $4.67 \pm 0.62$ | $-1.85 \pm 0.44$ |
| 60204.08357 | $36.5 \pm 1.4$ | $55.1 \pm 1.2$ | $7.24 \pm 0.89$ | $10.9 \pm 1.1$ | $10.49 \pm 0.65$ | $5.11 \pm 0.60$ | $6.32 \pm 0.62$ | $3.16 \pm 0.44$ |
| 60207.14767 | $33.6 \pm 1.4$ | $59.8 \pm 1.2$ | $11.19 \pm 0.93$ | $14.1 \pm 1.3$ | $11.35 \pm 0.67$ | $6.04 \pm 0.62$ | $6.48 \pm 0.65$ | $1.44 \pm 0.45$ |
| 60207.15530 | $30.5 \pm 1.4$ | $57.6 \pm 1.2$ | $11.98 \pm 0.90$ | $16.9 \pm 1.1$ | $10.61 \pm 0.65$ | $5.27 \pm 0.59$ | $6.26 \pm 0.62$ | $1.13 \pm 0.43$ |
